# Supplementary material for: Incorporating Connectivity among Internet Search Data for Enhanced Influenza-like Illness Tracking
Source: arXiv:2308.10091 source file (2023-08-19)
Supplement: Supplementary file 1 [file supplement.tex]

\setcounter{page}{1}

\rfoot{\thepage}
\section*{Supplementary Materials}

\setcounter{table}{0}
\setcounter{figure}{0}

\begin{sidewaysfigure}[htbp]
\begin{adjustwidth}{-4.5cm}{-4.5cm}
\centering
\includegraphics[width=\textwidth]{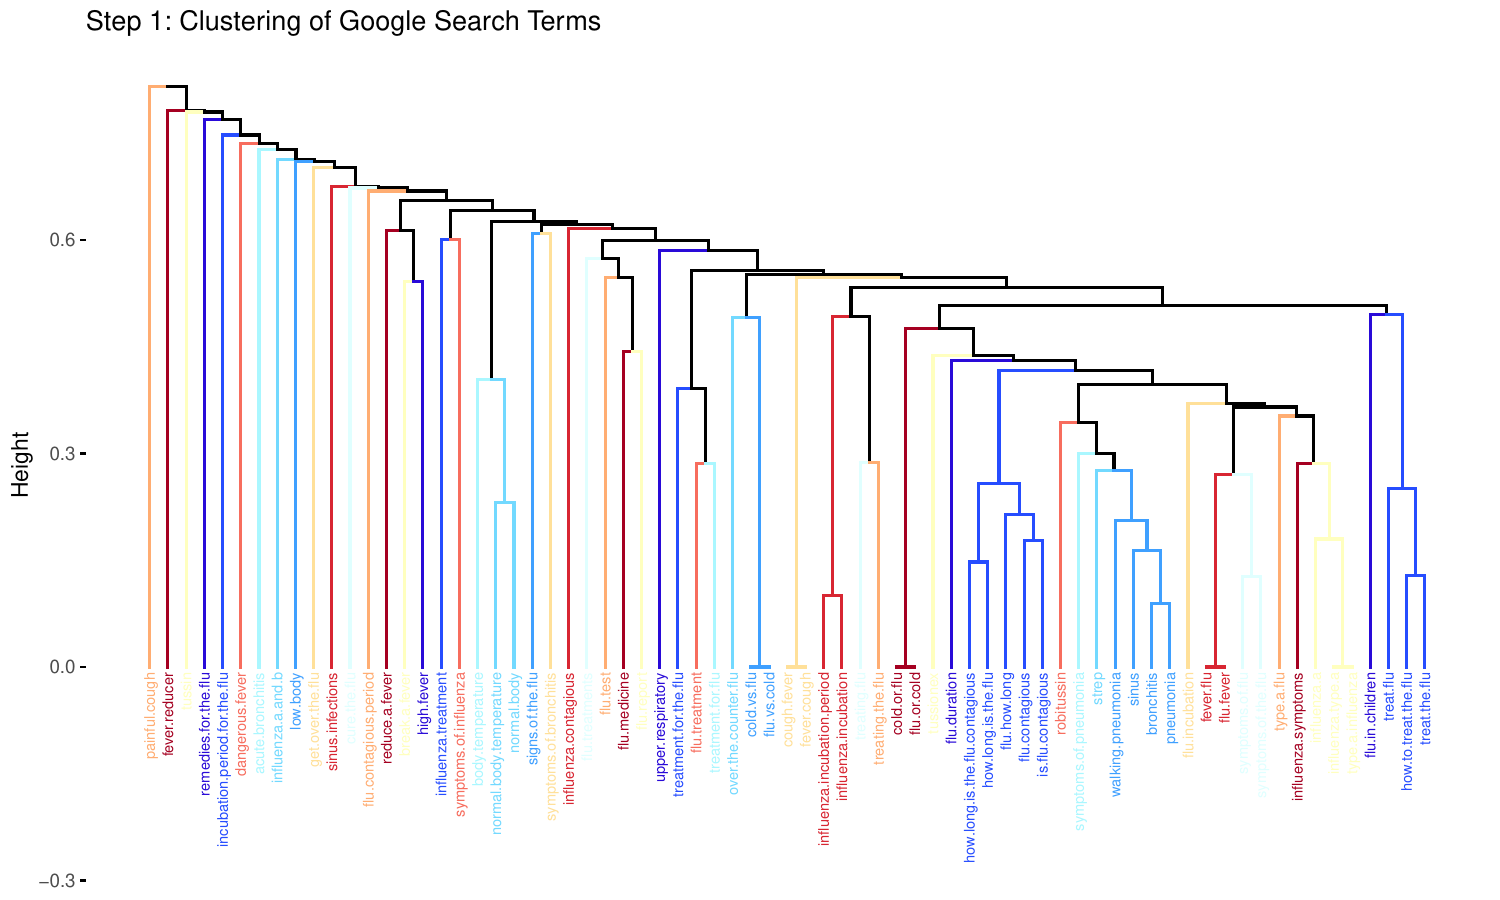}
\end{adjustwidth}
\caption{Clustering of the 71 Google search terms, collected by March 29, 2009. 53 clusters were identified. Hierarchical clustering with average linkage and correlation distance metric were used. The clustering was conducted based on the time series of Google search data from January 10, 2004 (the earliest available Google Trends data) to March 29, 2009 (the earliest prediction date by these 71 terms).}
\label{fig:pre09}
\end{sidewaysfigure}

\begin{sidewaysfigure}[htbp]
\begin{adjustwidth}{-4.5cm}{-4.5cm}
\centering
\includegraphics[width=1\textwidth]{{figs/fig\_clust\_hc\_corr\_ave\_post10}.pdf}
\end{adjustwidth}
\caption{Clustering of the 161 Google search terms, collected by May 22, 2010. 45 clusters were identified. Hierarchical clustering with average linkage and correlation distance metric were adopted. The clustering was conducted based on the time series of Google search data from January 10, 2004 (the earliest available Google Trends data) to May 22, 2010 (the earliest prediction date by these 161 terms).}
\label{fig:post10}
\end{sidewaysfigure}

\begin{figure}[!ht]
\centering
\includegraphics[width=0.6\textwidth]
{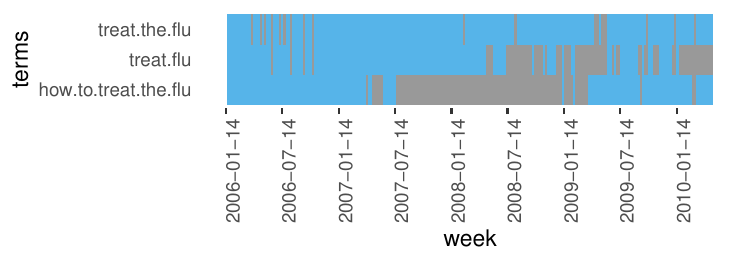}
\includegraphics[width=0.6\textwidth]
{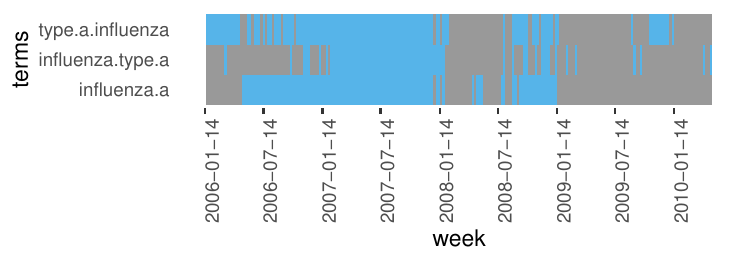}
\includegraphics[width=\textwidth]
{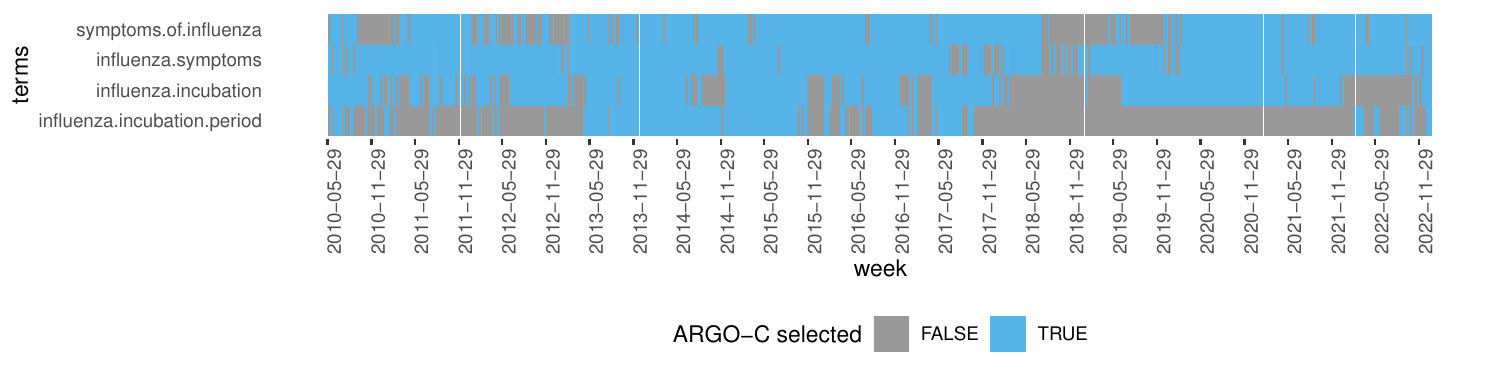}
\caption{Traceplots of clustered predictors included in the ARGO-C model at the national level over time. The heatmaps indicate whether each predictor was included in the predictive ARGO-C model at each week. Three exemplary clusters were highlighted. Each of the top two clusters contains three search terms (identified among 71 search terms by March 29, 2009, used for predictions before 2010), while the last one includes four search terms (identified among 161 topics/terms by May 22, 2010 and used for predictions since 2010). The entire cluster was penalized and excluded from the model when an entire column in the traceplot is colored grey.}\label{fig:traceplot_coef}
\end{figure}

\begin{table}[!ht]
\begin{adjustwidth}{-4.5cm}{-4cm}
\small
\centering
\begin{tabular}{c|llll}
  \hline
& Overall '09-'23 & '20-'21 & '21-'22 & '22-'23 \\ 
  \hline          
  \multicolumn{1}{l|}{RSME} \\
ARGO-C & \textbf{0.252} & 0.113 & \textbf{0.224} & 0.490 \\ 
  GFT & -- & -- & -- & -- \\ 
  VAR1 & 0.359 & \textbf{0.081} & 0.357 & 0.769 \\ 
  ARGO & 0.258 & 0.100 & 0.232 & \textbf{0.487} \\ 
  naive & 0.355 & 0.082 & 0.358 & 0.734 \\ 
   \hline
   \hline  \multicolumn{1}{l|}{MAE}\\
ARGO-C & 0.161 & 0.089 & 0.181 & 0.429 \\ 
  GFT & -- & -- & -- & -- \\ 
  VAR1 & 0.211 & \textbf{0.066} & 0.245 & 0.644 \\ 
  ARGO & \textbf{0.158} & 0.086 & \textbf{0.168} & \textbf{0.374} \\ 
  naive & 0.210 & 0.067 & 0.239 & 0.591 \\ 
   \hline  \multicolumn{1}{l|}{Correlation}\\ARGO-C & \textbf{0.984} & 0.927 & \textbf{0.983} & \textbf{0.975} \\ 
  GFT & -- & -- & -- & -- \\ 
  VAR1 & 0.968 & \textbf{0.941} & 0.899 & 0.909 \\ 
  ARGO & 0.983 & 0.940 & 0.962 & 0.969 \\ 
  naive & 0.968 & 0.939 & 0.900 & 0.907 \\ 

   \hline
\end{tabular}
\end{adjustwidth}
\caption{Comparison of \% ILI estimation between ARGO-C and other benchmarks at the national level, for flu seasons since COVID-19. The evaluation is based at the national level \%ILI in multiple periods and multiple metrics. RMSE, MAE, and correlation are reported. The method with the best performance is highlighted in boldface for each metric in each period. Methods considered here include ARGO-C, VAR1, GFT, the original ARGO, and the naive method. All comparisons are conducted on the original scale of the CDC’s \%ILI. The overall period '09-'23 is March 29, 2009 to January 28, 2023, including the period since COVID. Each regular flu season is from week 40 to week 20 next year, as defined by CDC’s Morbidity and Mortality Weekly Report. (The '22-'23 season is up to January 28, 2023).} \label{tab:covid}
\end{table}

\begin{table}[!ht]
\small
\centering
\begin{tabular}{c|lllll}
  \hline
  & Overall '14-'23 & post-COVID & '20-'21 & '21-'22 & '22-'23 \\ 
  \hline \hline \multicolumn{1}{l|}{RMSE}\\ARGO-C & \textbf{0.564} & \textbf{0.554} & 0.287 & \textbf{0.480} & \textbf{1.048} \\ 
  ARGOX & 0.576 & 0.574 & 0.283 & 0.488 & 1.101 \\ 
  VAR1 & 1.789 & 1.660 & 0.736 & 1.368 & 3.398 \\ 
  GFT & -- & -- & -- & -- & -- \\ 
  naive & 0.662 & 0.626 & \textbf{0.279} & 0.551 & 1.224 \\ 
   \hline \hline \multicolumn{1}{l|}{MAE}\\ARGO-C & \textbf{0.325} & \textbf{0.304} & 0.186 & 0.306 & \textbf{0.685} \\ 
  ARGOX & 0.329 & 0.309 & 0.182 & \textbf{0.305} & 0.735 \\ 
  VAR1 & 1.114 & 0.979 & 0.511 & 0.954 & 2.364 \\ 
  GFT & -- & -- & -- & -- & -- \\ 
  naive & 0.370 & 0.336 & \textbf{0.166} & 0.346 & 0.849 \\ 
   \hline \hline \multicolumn{1}{l|}{Correlation}\\ARGO-C & \textbf{0.947} & \textbf{0.933} & 0.703 & \textbf{0.862} & \textbf{0.890} \\ 
  ARGOX & 0.944 & 0.929 & 0.709 & 0.855 & 0.877 \\ 
  VAR1 & 0.675 & 0.719 & 0.478 & 0.563 & 0.591 \\ 
  GFT & -- & -- & -- & -- & -- \\ 
  naive & 0.929 & 0.919 & \textbf{0.710} & 0.816 & 0.844 \\ 
   \hline
\end{tabular}
\caption{Comparison of \% ILI estimation between ARGO-C and other benchmarks at the state level, for flu seasons since COVID-19. The evaluation is based on the average of 51 US state/district in multiple periods and multiple metrics. RMSE, MAE, and correlation are reported. The method with the best performance is highlighted in boldface for each metric in each period. Methods considered here include ARGO-C, VAR1, GFT, the original ARGOX, and the naive method. All comparisons are conducted on the original scale of the CDC’s \%ILI. The overall period '14-'23 is January 10, 2014 (first available estimate by ARGO framework) to January 28, 2023, including the period since COVID. The post-COVID period is the period since COVID, March 21, 2020 to  January 28, 2023. Each regular flu season is from week 40 to week 20 next year, as defined by CDC’s Morbidity and Mortality Weekly Report. (The '22-'23 season is up to January 28, 2023).} \label{tab:state_covid}
\end{table}

\begin{table}[!ht]
\centering
\begin{tabular}{rrrrrrrrrrrrrrr}
  \hline
AL & AK & AZ & AR & CA & CO & CT & DE & DC & GA & HI & ID & IL & IN & IA \\ 
0.931 & 0.926 & 0.915 & 0.929 & 0.947 & 0.903 & 0.906 & 0.947 & 0.908 & 0.933 & 0.942 & 0.933 & 0.931 & 0.924 & 0.931 \\ 
   \hline
   \hline
  KS & KY & LA & ME & MD & MA & MI & MN & MS & MO & MT & NE & NV & NH & NJ \\ 

0.938 & 0.894 & 0.922 & 0.917 & 0.933 & 0.919 & 0.940 & 0.942 & 0.938 & 0.935 & 0.935 & 0.910 & 0.903 & 0.908 & 0.929 \\    \hline
  \hline
NM & NY & NC & ND & OH & OK & OR & PA & RI & SC & SD & TN & TX & UT & VT \\ 

0.915 & 0.899 & 0.952 & 0.949 & 0.924 & 0.924 & 0.926 & 0.940 & 0.919 & 0.938 & 0.940 & 0.915 & 0.933 & 0.931 & 0.945 \\ 
   \hline
     \hline
VA & WA & WV & WI & WY & NYC \\ 
0.954 & 0.908 & 0.917 & 0.945 & 0.885 & 0.915 \\ 
   \hline
\end{tabular}
\caption{Actual coverage of prediction intervals by ARGO-C for state-level \%ILI prediction. The coverage is for 95\% nominal level. The average coverage over 51 states/city/district is 92.6\%. The evaluation period is January 10, 2014 to March 21, 2020, excluding the period with COVID-19 influence.} \label{tab:ci_state}
\end{table}

\begin{table}[!ht]
\begin{adjustwidth}{0cm}{0cm}
\footnotesize
\centering
\begin{tabular}{llll}
  \hline
    acute bronchitis & body temperature & break a fever & bronchitis \\ 
  cold or flu & cold vs flu & cough fever & cure the flu \\ 
  dangerous fever & fever cough & fever flu & fever reducer \\ 
  flu contagious period & flu contagious & flu duration & flu fever \\ 
  flu how long & flu in children & flu incubation & flu medicine \\ 
  flu or cold & flu report & flu test & flu treatment \\ 
  flu treatments & flu vs cold & get over the flu & high fever \\ 
  how long is the flu contagious & how long is the flu & how to treat the flu & incubation period for the flu \\ 
  influenza a and b & influenza a & influenza contagious & influenza incubation period \\ 
  influenza incubation & influenza symptoms & influenza treatment & influenza type a \\ 
  is flu contagious & low body & normal body temperature & normal body \\ 
  over the counter flu & painful cough & pneumonia & reduce a fever \\ 
  remedies for the flu & robitussin & signs of the flu & sinus infections \\ 
  sinus & strep & symptoms of bronchitis & symptoms of flu \\ 
  symptoms of influenza & symptoms of pneumonia & symptoms of the flu & treat flu \\ 
  treat the flu & treating flu & treating the flu & treatment for flu \\ 
  treatment for the flu & tussin & tussionex & type a flu \\ 
  type a influenza & upper respiratory & walking pneumonia &  \\ 
  \hline
  a influenza & braun thermoscan & chest cold & cold and flu \\ 
  cold versus flu & contagious flu & cure flu & do i have the flu \\ 
  ear thermometer & early flu symptoms & expectorant & exposed to flu \\ 
  fever breaks & fight the flu & flu a symptoms & flu and cold \\ 
  flu and fever & flu care & flu children & flu complications \\ 
  flu cough & flu germs & flu headache & flu how long are you contagious \\ 
  flu incubation period & flu lasts & flu length & flu recovery \\ 
  flu relief & flu remedies & flu remedy & flu reports \\ 
  flu symptoms & flu texas & flu versus cold & flu \\ 
  get rid of the flu & having the flu & how long am i contagious with the flu & how long contagious \\ 
  how long does flu last & how long does the flu last & how long flu & how long is flu contagious \\ 
  how to break a fever & how to bring a fever down & how to get rid of the flu & how to treat flu \\ 
  how to treat the flu at home & human temperature & i have the flu & incubation period for flu \\ 
  medicine for flu & medicine for the flu & oscillococcinum & over the counter flu medicine \\ 
  rapid flu & reduce fever & remedies for flu & respiratory flu \\ 
  signs of flu & strep throat & taking temperature & tessalon \\ 
  the flu virus & the flu & thermoscan & type a flu symptoms \\ 
  what to do if you have the flu &  &  &  \\ 
   \hline
  Influenza vaccine & Influenza & Fever & Influenza A virus \\ 
  Influenza B virus & Common cold & Cough & Sore throat \\ 
  Virus & Avian influenza & Spanish flu & Headache \\ 
  Nausea & Flu season & Oseltamivir & Nasal congestion \\ 
  Canine influenza & Rapid influenza diagnostic test & Theraflu & Dextromethorphan \\ 
  Rhinorrhea &  &  &  \\
   \hline
\end{tabular}
\caption{All search query terms used in this study. The first 71 terms were collected on March 29, 2009, the remaining terms/topics were identified on May 22, 2010. The last 21 terms separated by a horizontal line from the first 140 terms were ``Related topics'' from Google Trends.}\label{tab:query}
\end{adjustwidth}
\end{table}

\begin{table*}
\begin{adjustwidth}{0cm}{0cm}
\tiny
\centering
\begin{tabular}{c|llllllllllllllll}
  \hline
  & '09-'23 & '09-'15 & '09-'10 & '10-'11 & '11-'12 & '12-'13 & '13-'14 & '14-'15 & '15-'16 & '16-'17 & '17-'18 & '18-'19 & '19-'20 & '20-'21 & '21-'22 & '22-'23 \\ 
  \hline \hline \multicolumn{1}{l}{RMSE}\\ARGO-C & \textbf{0.307} & \textbf{0.349} & 0.903 & 0.174 & 0.115 & \textbf{0.253} & \textbf{0.214} & \textbf{0.321} & \textbf{0.183} & \textbf{0.214} & \textbf{0.256} & \textbf{0.180} & \textbf{0.432} & 0.092 & \textbf{0.297} & \textbf{0.784} \\ 
  ARGO2 & 0.316 & 0.353 & 0.904 & \textbf{0.172} & 0.104 & 0.284 & 0.216 & 0.330 & 0.190 & 0.225 & 0.273 & 0.187 & 0.450 & 0.096 & 0.306 & 0.829 \\ 
  VAR1 & 0.382 & 0.409 & 1.069 & 0.194 & \textbf{0.104} & 0.372 & 0.214 & 0.371 & 0.212 & 0.276 & 0.440 & 0.271 & 0.636 & \textbf{0.067} & 0.365 & 1.011 \\ 
  GFT & -- & 0.941 & \textbf{0.466} & 0.237 & 0.245 & 2.819 & 0.395 & 0.418 & -- & -- & -- & -- & -- & -- & -- & -- \\ 
  naive & 0.377 & 0.406 & 1.062 & 0.193 & 0.105 & 0.362 & 0.214 & 0.360 & 0.213 & 0.264 & 0.436 & 0.271 & 0.628 & 0.068 & 0.360 & 0.970 \\ 
   \hline \hline \multicolumn{1}{l}{MAE}\\ARGO-C & \textbf{0.164} & \textbf{0.169} & 0.486 & 0.133 & 0.095 & \textbf{0.157} & \textbf{0.171} & \textbf{0.203} & \textbf{0.141} & \textbf{0.169} & \textbf{0.186} & \textbf{0.141} & \textbf{0.300} & 0.069 & \textbf{0.209} & \textbf{0.548} \\ 
  ARGO2 & 0.168 & 0.171 & 0.487 & \textbf{0.127} & 0.087 & 0.163 & 0.178 & 0.204 & 0.147 & 0.173 & 0.188 & 0.145 & 0.306 & 0.076 & 0.221 & 0.597 \\ 
  VAR1 & 0.198 & 0.187 & 0.569 & 0.147 & \textbf{0.086} & 0.221 & 0.182 & 0.213 & 0.170 & 0.199 & 0.323 & 0.186 & 0.488 & \textbf{0.052} & 0.282 & 0.725 \\ 
  GFT & -- & 0.327 & \textbf{0.267} & 0.195 & 0.176 & 1.330 & 0.334 & 0.322 & -- & -- & -- & -- & -- & -- & -- & -- \\ 
  naive & 0.198 & 0.188 & 0.583 & 0.143 & 0.087 & 0.224 & 0.180 & 0.221 & 0.165 & 0.193 & 0.324 & 0.192 & 0.497 & 0.053 & 0.278 & 0.690 \\ 
   \hline \hline \multicolumn{1}{l}{Correlation}\\ARGO-C & \textbf{0.968} & \textbf{0.934} & 0.913 & \textbf{0.956} & 0.630 & \textbf{0.960} & \textbf{0.885} & \textbf{0.931} & \textbf{0.938} & \textbf{0.964} & \textbf{0.984} & \textbf{0.983} & \textbf{0.975} & 0.949 & \textbf{0.931} & \textbf{0.943} \\ 
  ARGO2 & 0.966 & 0.933 & 0.913 & 0.955 & 0.690 & 0.951 & 0.880 & 0.929 & 0.933 & 0.960 & 0.983 & 0.982 & 0.975 & \textbf{0.951} & 0.923 & 0.935 \\ 
  VAR1 & 0.949 & 0.909 & 0.876 & 0.931 & 0.689 & 0.915 & 0.882 & 0.907 & 0.921 & 0.929 & 0.951 & 0.961 & 0.942 & 0.948 & 0.888 & 0.900 \\ 
  GFT & -- & 0.768 & \textbf{0.988} & 0.911 & \textbf{0.699} & 0.831 & 0.786 & 0.917 & -- & -- & -- & -- & -- & -- & -- & -- \\ 
  naive & 0.951 & 0.914 & 0.884 & 0.932 & 0.693 & 0.919 & 0.884 & 0.914 & 0.923 & 0.936 & 0.951 & 0.961 & 0.944 & 0.947 & 0.892 & 0.899 \\ 
   \hline
\end{tabular}
\caption{Comparison of different methods for regional level \%ILI estimation in Region 1. The RMSE, MAE, and correlation measures are reported. The method with the best performance is highlighted in boldface for each metric in each period. \label{tab:reg1}} 
\end{adjustwidth}\end{table*}

\begin{table*}
\begin{adjustwidth}{0cm}{0cm}
\tiny
\centering
\begin{tabular}{c|llllllllllllllll}
  \hline
  & '09-'23 & '09-'15 & '09-'10 & '10-'11 & '11-'12 & '12-'13 & '13-'14 & '14-'15 & '15-'16 & '16-'17 & '17-'18 & '18-'19 & '19-'20 & '20-'21 & '21-'22 & '22-'23 \\ 
  \hline \hline \multicolumn{1}{l}{RMSE}\\ARGO-C & \textbf{0.446} & \textbf{0.418} & 0.646 & \textbf{0.385} & 0.134 & \textbf{0.340} & 0.337 & \textbf{0.374} & 0.354 & \textbf{0.540} & 0.599 & \textbf{0.228} & 0.953 & 0.229 & \textbf{0.552} & \textbf{0.885} \\ 
  ARGO2 & 0.458 & 0.430 & 0.647 & 0.394 & 0.125 & 0.395 & \textbf{0.330} & 0.415 & \textbf{0.352} & 0.577 & \textbf{0.588} & 0.241 & \textbf{0.929} & 0.230 & 0.579 & 0.990 \\ 
  VAR1 & 0.544 & 0.480 & 0.793 & 0.415 & \textbf{0.120} & 0.498 & 0.366 & 0.496 & 0.372 & 0.639 & 0.880 & 0.333 & 1.250 & \textbf{0.222} & 0.665 & 1.078 \\ 
  GFT & -- & 1.037 & \textbf{0.463} & 1.093 & 0.510 & 2.370 & 0.665 & 0.662 & -- & -- & -- & -- & -- & -- & -- & -- \\ 
  naive & 0.541 & 0.482 & 0.799 & 0.421 & 0.121 & 0.498 & 0.367 & 0.489 & 0.381 & 0.627 & 0.868 & 0.333 & 1.229 & 0.225 & 0.667 & 1.047 \\ 
   \hline \hline \multicolumn{1}{l}{MAE}\\ARGO-C & \textbf{0.280} & \textbf{0.268} & 0.430 & \textbf{0.272} & 0.110 & \textbf{0.242} & 0.285 & \textbf{0.314} & \textbf{0.292} & \textbf{0.442} & \textbf{0.429} & \textbf{0.186} & \textbf{0.567} & \textbf{0.174} & \textbf{0.412} & \textbf{0.626} \\ 
  ARGO2 & 0.288 & 0.275 & 0.434 & 0.282 & 0.101 & 0.260 & \textbf{0.283} & 0.345 & 0.296 & 0.460 & 0.439 & 0.193 & 0.575 & 0.177 & 0.417 & 0.684 \\ 
  VAR1 & 0.325 & 0.293 & 0.450 & 0.313 & \textbf{0.097} & 0.347 & 0.308 & 0.355 & 0.307 & 0.462 & 0.577 & 0.274 & 0.896 & 0.177 & 0.462 & 0.822 \\ 
  GFT & -- & 0.632 & \textbf{0.364} & 0.936 & 0.440 & 1.310 & 0.611 & 0.487 & -- & -- & -- & -- & -- & -- & -- & -- \\ 
  naive & 0.323 & 0.297 & 0.460 & 0.304 & 0.097 & 0.358 & 0.309 & 0.360 & 0.301 & 0.449 & 0.572 & 0.275 & 0.879 & 0.180 & 0.442 & 0.796 \\ 
   \hline \hline \multicolumn{1}{l}{Correlation}\\ARGO-C & \textbf{0.969} & \textbf{0.950} & 0.944 & \textbf{0.938} & 0.664 & \textbf{0.968} & 0.848 & \textbf{0.951} & 0.921 & \textbf{0.946} & 0.971 & \textbf{0.974} & 0.950 & \textbf{0.768} & \textbf{0.916} & \textbf{0.937} \\ 
  ARGO2 & 0.968 & 0.947 & 0.946 & 0.934 & \textbf{0.693} & 0.959 & 0.849 & 0.945 & \textbf{0.922} & 0.936 & \textbf{0.974} & 0.971 & \textbf{0.958} & 0.767 & 0.903 & 0.921 \\ 
  VAR1 & 0.952 & 0.934 & 0.912 & 0.927 & 0.678 & 0.930 & 0.831 & 0.907 & 0.902 & 0.912 & 0.940 & 0.944 & 0.901 & 0.765 & 0.866 & 0.878 \\ 
  GFT & -- & 0.783 & \textbf{0.981} & 0.870 & 0.398 & 0.915 & \textbf{0.871} & 0.932 & -- & -- & -- & -- & -- & -- & -- & -- \\ 
  naive & 0.954 & 0.935 & 0.914 & 0.927 & 0.684 & 0.931 & 0.831 & 0.910 & 0.902 & 0.917 & 0.940 & 0.945 & 0.904 & 0.763 & 0.867 & 0.883 \\ 
   \hline
\end{tabular}
\caption{Comparison of different methods for regional level \%ILI estimation in Region 2.  The RMSE, MAE, and correlation measures are reported. The method with the best performance is highlighted in boldface for each metric in each period. \label{tab:reg2}} 
\end{adjustwidth}\end{table*}

% latex table generated in R 4.0.1 by xtable 1.8-4 package
% Tue May  2 13:07:15 2023

\begin{table*}\begin{adjustwidth}{0cm}{0cm} \tiny
\centering
\begin{tabular}{c|llllllllllllllll}
  \hline
  & '09-'23 & '09-'15 & '09-'10 & '10-'11 & '11-'12 & '12-'13 & '13-'14 & '14-'15 & '15-'16 & '16-'17 & '17-'18 & '18-'19 & '19-'20 & '20-'21 & '21-'22 & '22-'23 \\ 
  \hline \hline \multicolumn{1}{l}{RMSE}\\ARGO-C & \textbf{0.324} & \textbf{0.393} & 0.755 & \textbf{0.264} & \textbf{0.175} & \textbf{0.597} & \textbf{0.230} & 0.458 & \textbf{0.219} & \textbf{0.367} & \textbf{0.379} & \textbf{0.194} & \textbf{0.295} & 0.128 & \textbf{0.303} & \textbf{0.500} \\ 
  ARGO2 & 0.350 & 0.425 & 0.799 & 0.291 & 0.181 & 0.667 & 0.243 & 0.539 & 0.232 & 0.403 & 0.381 & 0.217 & 0.342 & 0.125 & 0.335 & 0.564 \\ 
  VAR1 & 0.460 & 0.522 & 0.998 & 0.327 & 0.193 & 0.786 & 0.311 & 0.745 & 0.320 & 0.530 & 0.652 & 0.334 & 0.708 & \textbf{0.104} & 0.450 & 0.698 \\ 
  GFT & -- & 0.859 & \textbf{0.604} & 0.501 & 0.926 & 2.188 & 0.514 & \textbf{0.380} & -- & -- & -- & -- & -- & -- & -- & -- \\ 
  naive & 0.457 & 0.522 & 0.993 & 0.337 & 0.196 & 0.785 & 0.312 & 0.745 & 0.323 & 0.506 & 0.645 & 0.329 & 0.699 & 0.106 & 0.454 & 0.673 \\ 
   \hline \hline \multicolumn{1}{l}{MAE}\\ARGO-C & \textbf{0.201} & \textbf{0.241} & \textbf{0.458} & \textbf{0.208} & \textbf{0.143} & \textbf{0.396} & \textbf{0.173} & \textbf{0.286} & \textbf{0.176} & \textbf{0.277} & \textbf{0.272} & \textbf{0.152} & \textbf{0.218} & 0.092 & \textbf{0.209} & \textbf{0.361} \\ 
  ARGO2 & 0.213 & 0.255 & 0.484 & 0.237 & 0.143 & 0.421 & 0.188 & 0.339 & 0.178 & 0.306 & 0.293 & 0.173 & 0.249 & 0.097 & 0.214 & 0.396 \\ 
  VAR1 & 0.258 & 0.282 & 0.555 & 0.245 & 0.153 & 0.477 & 0.204 & 0.410 & 0.254 & 0.336 & 0.407 & 0.269 & 0.512 & \textbf{0.080} & 0.284 & 0.594 \\ 
  GFT & -- & 0.567 & 0.474 & 0.428 & 0.886 & 1.760 & 0.480 & 0.312 & -- & -- & -- & -- & -- & -- & -- & -- \\ 
  naive & 0.258 & 0.286 & 0.555 & 0.256 & 0.153 & 0.482 & 0.210 & 0.430 & 0.260 & 0.319 & 0.411 & 0.262 & 0.513 & 0.081 & 0.281 & 0.548 \\ 
   \hline \hline \multicolumn{1}{l}{Correlation}\\ARGO-C & \textbf{0.973} & \textbf{0.957} & 0.960 & \textbf{0.975} & 0.725 & \textbf{0.916} & \textbf{0.975} & 0.964 & \textbf{0.939} & \textbf{0.961} & 0.984 & \textbf{0.991} & \textbf{0.988} & 0.922 & \textbf{0.954} & \textbf{0.952} \\ 
  ARGO2 & 0.969 & 0.951 & 0.955 & 0.969 & 0.712 & 0.894 & 0.974 & 0.954 & 0.936 & 0.953 & \textbf{0.986} & 0.989 & 0.986 & \textbf{0.932} & 0.935 & 0.938 \\ 
  VAR1 & 0.944 & 0.923 & 0.924 & 0.950 & 0.671 & 0.852 & 0.924 & 0.886 & 0.868 & 0.905 & 0.944 & 0.960 & 0.924 & 0.928 & 0.866 & 0.891 \\ 
  GFT & -- & 0.865 & \textbf{0.991} & 0.953 & \textbf{0.732} & 0.891 & 0.975 & \textbf{0.985} & -- & -- & -- & -- & -- & -- & -- & -- \\ 
  naive & 0.946 & 0.925 & 0.927 & 0.947 & 0.676 & 0.859 & 0.926 & 0.891 & 0.870 & 0.916 & 0.945 & 0.962 & 0.927 & 0.927 & 0.866 & 0.892 \\ 
   \hline
\end{tabular}
\caption{Comparison of different methods for regional level \%ILI estimation in Region 3.  The RMSE, MAE, and correlation measures are reported. The method with the best performance is highlighted in boldface for each metric in each period. \label{tab:reg3}} 
\end{adjustwidth}\end{table*}
% latex table generated in R 4.0.1 by xtable 1.8-4 package
% Tue May  2 13:07:15 2023
\begin{table*}\begin{adjustwidth}{0cm}{0cm} \tiny
\centering
\begin{tabular}{c|llllllllllllllll}
  \hline
  & '09-'23 & '09-'15 & '09-'10 & '10-'11 & '11-'12 & '12-'13 & '13-'14 & '14-'15 & '15-'16 & '16-'17 & '17-'18 & '18-'19 & '19-'20 & '20-'21 & '21-'22 & '22-'23 \\ 
  \hline \hline \multicolumn{1}{l}{RMSE}\\ARGO-C & \textbf{0.335} & \textbf{0.356} & 0.313 & \textbf{0.377} & \textbf{0.180} & 0.524 & \textbf{0.243} & 0.476 & \textbf{0.179} & \textbf{0.390} & 0.421 & \textbf{0.239} & \textbf{0.531} & 0.139 & \textbf{0.286} & \textbf{0.726} \\ 
  ARGO2 & 0.353 & 0.357 & \textbf{0.276} & 0.394 & 0.192 & \textbf{0.524} & 0.267 & 0.517 & 0.210 & 0.415 & \textbf{0.418} & 0.300 & 0.662 & 0.141 & 0.321 & 0.776 \\ 
  VAR1 & 0.463 & 0.422 & 0.286 & 0.477 & 0.203 & 0.568 & 0.386 & 0.728 & 0.281 & 0.505 & 0.817 & 0.483 & 0.923 & \textbf{0.098} & 0.466 & 0.994 \\ 
  GFT & -- & 0.821 & 0.522 & 0.908 & 0.270 & 2.023 & 0.407 & \textbf{0.358} & -- & -- & -- & -- & -- & -- & -- & -- \\ 
  naive & 0.460 & 0.423 & 0.312 & 0.484 & 0.205 & 0.569 & 0.387 & 0.734 & 0.275 & 0.482 & 0.809 & 0.492 & 0.916 & 0.100 & 0.465 & 0.958 \\ 
   \hline \hline \multicolumn{1}{l}{MAE}\\ARGO-C & \textbf{0.204} & \textbf{0.205} & 0.225 & \textbf{0.291} & 0.139 & \textbf{0.325} & \textbf{0.166} & 0.278 & \textbf{0.153} & \textbf{0.297} & 0.284 & \textbf{0.168} & \textbf{0.398} & 0.119 & \textbf{0.206} & \textbf{0.456} \\ 
  ARGO2 & 0.214 & 0.206 & \textbf{0.213} & 0.309 & \textbf{0.138} & 0.329 & 0.172 & 0.298 & 0.171 & 0.327 & \textbf{0.276} & 0.211 & 0.468 & 0.126 & 0.219 & 0.505 \\ 
  VAR1 & 0.267 & 0.234 & 0.219 & 0.357 & 0.158 & 0.351 & 0.241 & 0.416 & 0.208 & 0.386 & 0.529 & 0.367 & 0.699 & \textbf{0.080} & 0.308 & 0.790 \\ 
  GFT & -- & 0.474 & 0.462 & 0.740 & 0.233 & 1.468 & 0.319 & \textbf{0.255} & -- & -- & -- & -- & -- & -- & -- & -- \\ 
  naive & 0.268 & 0.238 & 0.235 & 0.365 & 0.157 & 0.363 & 0.244 & 0.428 & 0.206 & 0.368 & 0.520 & 0.383 & 0.695 & 0.082 & 0.308 & 0.751 \\ 
   \hline \hline \multicolumn{1}{l}{Correlation}\\ARGO-C & \textbf{0.977} & \textbf{0.963} & 0.986 & 0.966 & \textbf{0.830} & \textbf{0.931} & 0.973 & 0.950 & \textbf{0.978} & \textbf{0.963} & 0.987 & \textbf{0.985} & \textbf{0.974} & 0.880 & \textbf{0.973} & \textbf{0.919} \\ 
  ARGO2 & 0.975 & 0.962 & \textbf{0.987} & 0.962 & 0.806 & 0.923 & 0.967 & 0.945 & 0.974 & 0.959 & \textbf{0.988} & 0.975 & 0.958 & 0.882 & 0.960 & 0.907 \\ 
  VAR1 & 0.957 & 0.947 & 0.986 & 0.945 & 0.792 & 0.907 & 0.920 & 0.880 & 0.926 & 0.931 & 0.952 & 0.931 & 0.908 & \textbf{0.919} & 0.904 & 0.844 \\ 
  GFT & -- & 0.835 & 0.984 & \textbf{0.975} & 0.771 & 0.892 & \textbf{0.977} & \textbf{0.979} & -- & -- & -- & -- & -- & -- & -- & -- \\ 
  naive & 0.958 & 0.948 & 0.986 & 0.944 & 0.793 & 0.909 & 0.922 & 0.881 & 0.929 & 0.937 & 0.951 & 0.930 & 0.911 & 0.916 & 0.906 & 0.847 \\ 
   \hline
\end{tabular}
\caption{Comparison of different methods for regional level \%ILI estimation in Region 4.  The RMSE, MAE, and correlation measures are reported. The method with the best performance is highlighted in boldface for each metric in each period. \label{tab:reg4}} 
\end{adjustwidth}\end{table*}
% latex table generated in R 4.0.1 by xtable 1.8-4 package
% Tue May  2 13:07:15 2023
\begin{table*}\begin{adjustwidth}{0cm}{0cm} \tiny
\centering
\begin{tabular}{c|llllllllllllllll}
  \hline
  & '09-'23 & '09-'15 & '09-'10 & '10-'11 & '11-'12 & '12-'13 & '13-'14 & '14-'15 & '15-'16 & '16-'17 & '17-'18 & '18-'19 & '19-'20 & '20-'21 & '21-'22 & '22-'23 \\ 
  \hline \hline \multicolumn{1}{l}{RMSE}\\ARGO-C & \textbf{0.275} & \textbf{0.326} & 0.729 & \textbf{0.241} & \textbf{0.162} & \textbf{0.378} & \textbf{0.197} & 0.388 & \textbf{0.161} & \textbf{0.267} & \textbf{0.201} & 0.233 & \textbf{0.381} & 0.094 & \textbf{0.247} & \textbf{0.534} \\ 
  ARGO2 & 0.296 & 0.347 & 0.776 & 0.262 & 0.176 & 0.404 & 0.220 & 0.425 & 0.179 & 0.283 & 0.219 & \textbf{0.233} & 0.448 & 0.099 & 0.259 & 0.605 \\ 
  VAR1 & 0.381 & 0.431 & 0.932 & 0.304 & 0.202 & 0.491 & 0.319 & 0.614 & 0.271 & 0.356 & 0.482 & 0.301 & 0.603 & \textbf{0.066} & 0.320 & 0.765 \\ 
  GFT & -- & 0.803 & \textbf{0.480} & 0.382 & 0.528 & 2.311 & 0.323 & \textbf{0.266} & -- & -- & -- & -- & -- & -- & -- & -- \\ 
  naive & 0.378 & 0.430 & 0.917 & 0.308 & 0.202 & 0.487 & 0.321 & 0.630 & 0.271 & 0.343 & 0.480 & 0.301 & 0.596 & 0.067 & 0.317 & 0.738 \\ 
   \hline \hline \multicolumn{1}{l}{MAE}\\ARGO-C & \textbf{0.159} & \textbf{0.178} & \textbf{0.410} & \textbf{0.183} & \textbf{0.134} & \textbf{0.243} & \textbf{0.121} & 0.225 & \textbf{0.116} & \textbf{0.201} & \textbf{0.154} & 0.169 & \textbf{0.261} & 0.077 & \textbf{0.179} & \textbf{0.410} \\ 
  ARGO2 & 0.166 & 0.185 & 0.433 & 0.190 & 0.141 & 0.251 & 0.125 & 0.258 & 0.128 & 0.202 & 0.166 & \textbf{0.167} & 0.304 & 0.084 & 0.187 & 0.463 \\ 
  VAR1 & 0.205 & 0.214 & 0.514 & 0.200 & 0.159 & 0.292 & 0.174 & 0.355 & 0.209 & 0.249 & 0.313 & 0.234 & 0.402 & \textbf{0.056} & 0.242 & 0.604 \\ 
  GFT & -- & 0.382 & 0.411 & 0.315 & 0.445 & 1.588 & 0.227 & \textbf{0.195} & -- & -- & -- & -- & -- & -- & -- & -- \\ 
  naive & 0.205 & 0.218 & 0.505 & 0.210 & 0.157 & 0.314 & 0.183 & 0.367 & 0.210 & 0.242 & 0.323 & 0.230 & 0.404 & 0.056 & 0.232 & 0.543 \\ 
   \hline \hline \multicolumn{1}{l}{Correlation}\\ARGO-C & \textbf{0.973} & \textbf{0.962} & 0.953 & \textbf{0.973} & \textbf{0.891} & \textbf{0.951} & 0.960 & 0.954 & \textbf{0.965} & \textbf{0.970} & \textbf{0.992} & 0.952 & \textbf{0.968} & 0.902 & \textbf{0.952} & \textbf{0.958} \\ 
  ARGO2 & 0.970 & 0.957 & 0.948 & 0.966 & 0.871 & 0.945 & 0.950 & 0.947 & 0.961 & 0.968 & 0.991 & \textbf{0.953} & 0.954 & 0.902 & 0.935 & 0.944 \\ 
  VAR1 & 0.949 & 0.933 & 0.922 & 0.947 & 0.835 & 0.918 & 0.882 & 0.882 & 0.894 & 0.936 & 0.952 & 0.918 & 0.911 & \textbf{0.931} & 0.879 & 0.902 \\ 
  GFT & -- & 0.879 & \textbf{0.985} & 0.938 & 0.709 & 0.906 & \textbf{0.964} & \textbf{0.988} & -- & -- & -- & -- & -- & -- & -- & -- \\ 
  naive & 0.950 & 0.934 & 0.924 & 0.947 & 0.837 & 0.920 & 0.883 & 0.880 & 0.897 & 0.940 & 0.952 & 0.920 & 0.915 & 0.929 & 0.881 & 0.901 \\ 
   \hline
\end{tabular}
\caption{Comparison of different methods for regional level \%ILI estimation in Region 5.  The RMSE, MAE, and correlation measures are reported. The method with the best performance is highlighted in boldface for each metric in each period. \label{tab:reg5}} 
\end{adjustwidth}\end{table*}
% latex table generated in R 4.0.1 by xtable 1.8-4 package
% Tue May  2 13:07:15 2023
\begin{table*}\begin{adjustwidth}{0cm}{0cm} \tiny
\centering
\begin{tabular}{c|llllllllllllllll}
  \hline
  & '09-'23 & '09-'15 & '09-'10 & '10-'11 & '11-'12 & '12-'13 & '13-'14 & '14-'15 & '15-'16 & '16-'17 & '17-'18 & '18-'19 & '19-'20 & '20-'21 & '21-'22 & '22-'23 \\ 
  \hline \hline \multicolumn{1}{l}{RMSE}\\ARGO-C & \textbf{0.557} & \textbf{0.615} & 0.893 & \textbf{0.466} & \textbf{0.239} & \textbf{0.541} & \textbf{0.548} & 1.117 & 0.362 & \textbf{0.593} & 0.803 & \textbf{0.517} & \textbf{1.017} & 0.298 & 0.311 & \textbf{0.625} \\ 
  ARGO2 & 0.578 & 0.631 & \textbf{0.884} & 0.507 & 0.273 & 0.612 & 0.572 & \textbf{1.108} & \textbf{0.362} & 0.647 & \textbf{0.763} & 0.553 & 1.144 & 0.314 & \textbf{0.303} & 0.663 \\ 
  VAR1 & 0.685 & 0.713 & 0.977 & 0.664 & 0.309 & 0.759 & 0.759 & 1.160 & 0.441 & 0.762 & 1.143 & 0.795 & 1.315 & \textbf{0.249} & 0.451 & 0.785 \\ 
  GFT & -- & 1.356 & 0.899 & 0.639 & 0.908 & 3.607 & 0.770 & 1.146 & -- & -- & -- & -- & -- & -- & -- & -- \\ 
  naive & 0.678 & 0.708 & 1.012 & 0.665 & 0.306 & 0.770 & 0.747 & 1.164 & 0.444 & 0.727 & 1.131 & 0.791 & 1.300 & 0.251 & 0.456 & 0.753 \\ 
   \hline \hline \multicolumn{1}{l}{MAE}\\ARGO-C & \textbf{0.338} & \textbf{0.370} & 0.593 & \textbf{0.366} & \textbf{0.175} & \textbf{0.407} & \textbf{0.361} & \textbf{0.627} & 0.300 & \textbf{0.399} & \textbf{0.424} & \textbf{0.353} & \textbf{0.707} & 0.240 & 0.222 & \textbf{0.499} \\ 
  ARGO2 & 0.352 & 0.385 & \textbf{0.579} & 0.402 & 0.188 & 0.442 & 0.368 & 0.678 & \textbf{0.293} & 0.417 & 0.441 & 0.373 & 0.788 & 0.250 & \textbf{0.220} & 0.542 \\ 
  VAR1 & 0.410 & 0.421 & 0.580 & 0.477 & 0.212 & 0.506 & 0.493 & 0.732 & 0.364 & 0.555 & 0.759 & 0.608 & 0.978 & \textbf{0.164} & 0.304 & 0.648 \\ 
  GFT & -- & 0.714 & 0.618 & 0.439 & 0.848 & 2.567 & 0.544 & 0.661 & -- & -- & -- & -- & -- & -- & -- & -- \\ 
  naive & 0.411 & 0.424 & 0.625 & 0.461 & 0.207 & 0.534 & 0.498 & 0.752 & 0.359 & 0.544 & 0.750 & 0.618 & 0.983 & 0.168 & 0.323 & 0.624 \\ 
   \hline \hline \multicolumn{1}{l}{Correlation}\\ARGO-C & \textbf{0.973} & \textbf{0.959} & 0.961 & 0.974 & 0.909 & \textbf{0.967} & \textbf{0.963} & 0.896 & \textbf{0.890} & \textbf{0.972} & 0.981 & \textbf{0.984} & \textbf{0.954} & \textbf{0.691} & \textbf{0.949} & \textbf{0.952} \\ 
  ARGO2 & 0.971 & 0.958 & 0.962 & 0.969 & 0.879 & 0.958 & 0.959 & 0.899 & 0.886 & 0.968 & \textbf{0.982} & 0.980 & 0.942 & 0.675 & 0.946 & 0.947 \\ 
  VAR1 & 0.958 & 0.945 & 0.952 & 0.943 & 0.850 & 0.934 & 0.924 & 0.890 & 0.833 & 0.944 & 0.957 & 0.947 & 0.916 & 0.684 & 0.878 & 0.911 \\ 
  GFT & -- & 0.878 & \textbf{0.980} & \textbf{0.978} & \textbf{0.914} & 0.943 & 0.956 & \textbf{0.928} & -- & -- & -- & -- & -- & -- & -- & -- \\ 
  naive & 0.960 & 0.947 & 0.954 & 0.944 & 0.855 & 0.933 & 0.927 & 0.893 & 0.837 & 0.950 & 0.957 & 0.949 & 0.920 & 0.681 & 0.877 & 0.916 \\ 
   \hline
\end{tabular}
\caption{Comparison of different methods for regional level \%ILI estimation in Region 6.  The RMSE, MAE, and correlation measures are reported. The method with the best performance is highlighted in boldface for each metric in each period. \label{tab:reg6}} 
\end{adjustwidth}\end{table*}
% latex table generated in R 4.0.1 by xtable 1.8-4 package
% Tue May  2 13:07:15 2023
\begin{table*}\begin{adjustwidth}{0cm}{0cm} \tiny
\centering
\begin{tabular}{c|llllllllllllllll}
  \hline
  & '09-'23 & '09-'15 & '09-'10 & '10-'11 & '11-'12 & '12-'13 & '13-'14 & '14-'15 & '15-'16 & '16-'17 & '17-'18 & '18-'19 & '19-'20 & '20-'21 & '21-'22 & '22-'23 \\ 
  \hline \hline \multicolumn{1}{l}{RMSE}\\ARGO-C & \textbf{0.423} & \textbf{0.463} & \textbf{0.921} & \textbf{0.387} & \textbf{0.298} & \textbf{0.470} & \textbf{0.263} & \textbf{0.377} & \textbf{0.211} & \textbf{0.448} & \textbf{0.461} & \textbf{0.487} & \textbf{0.584} & 0.260 & 0.268 & \textbf{0.781} \\ 
  ARGO2 & 0.453 & 0.493 & 0.969 & 0.402 & 0.324 & 0.535 & 0.309 & 0.459 & 0.212 & 0.489 & 0.510 & 0.515 & 0.709 & 0.266 & \textbf{0.255} & 0.840 \\ 
  VAR1 & 0.552 & 0.572 & 1.122 & 0.491 & 0.348 & 0.631 & 0.459 & 0.621 & 0.245 & 0.583 & 0.908 & 0.656 & 0.917 & \textbf{0.231} & 0.305 & 1.006 \\ 
  GFT & -- & 0.917 & 1.968 & 1.077 & 0.603 & 0.718 & 0.322 & 0.856 & -- & -- & -- & -- & -- & -- & -- & -- \\ 
  naive & 0.546 & 0.569 & 1.111 & 0.495 & 0.343 & 0.637 & 0.468 & 0.623 & 0.246 & 0.555 & 0.903 & 0.651 & 0.903 & 0.236 & 0.312 & 0.964 \\ 
   \hline \hline \multicolumn{1}{l}{MAE}\\ARGO-C & \textbf{0.244} & \textbf{0.261} & \textbf{0.600} & \textbf{0.302} & \textbf{0.229} & \textbf{0.290} & \textbf{0.179} & \textbf{0.242} & 0.166 & \textbf{0.300} & \textbf{0.314} & \textbf{0.357} & \textbf{0.405} & 0.140 & 0.205 & \textbf{0.481} \\ 
  ARGO2 & 0.260 & 0.280 & 0.641 & 0.312 & 0.242 & 0.313 & 0.203 & 0.302 & \textbf{0.164} & 0.319 & 0.342 & 0.375 & 0.488 & 0.157 & \textbf{0.186} & 0.516 \\ 
  VAR1 & 0.300 & 0.304 & 0.698 & 0.346 & 0.262 & 0.365 & 0.278 & 0.376 & 0.200 & 0.404 & 0.595 & 0.481 & 0.630 & \textbf{0.116} & 0.214 & 0.705 \\ 
  GFT & -- & 0.506 & 1.385 & 0.791 & 0.436 & 0.539 & 0.200 & 0.493 & -- & -- & -- & -- & -- & -- & -- & -- \\ 
  naive & 0.303 & 0.313 & 0.716 & 0.354 & 0.259 & 0.390 & 0.298 & 0.412 & 0.195 & 0.397 & 0.600 & 0.467 & 0.630 & 0.119 & 0.224 & 0.658 \\ 
   \hline \hline \multicolumn{1}{l}{Correlation}\\ARGO-C & \textbf{0.969} & \textbf{0.959} & 0.943 & 0.953 & 0.941 & \textbf{0.961} & \textbf{0.970} & \textbf{0.975} & 0.901 & \textbf{0.961} & \textbf{0.988} & \textbf{0.958} & \textbf{0.970} & 0.798 & \textbf{0.963} & \textbf{0.931} \\ 
  ARGO2 & 0.965 & 0.955 & 0.938 & 0.949 & 0.931 & 0.952 & 0.960 & 0.967 & \textbf{0.903} & 0.954 & 0.986 & 0.953 & 0.955 & 0.792 & 0.956 & 0.918 \\ 
  VAR1 & 0.946 & 0.936 & 0.913 & 0.916 & 0.917 & 0.929 & 0.899 & 0.921 & 0.855 & 0.930 & 0.951 & 0.913 & 0.924 & \textbf{0.817} & 0.928 & 0.876 \\ 
  GFT & -- & 0.846 & \textbf{0.985} & \textbf{0.960} & \textbf{0.953} & 0.934 & 0.964 & 0.963 & -- & -- & -- & -- & -- & -- & -- & -- \\ 
  naive & 0.948 & 0.938 & 0.918 & 0.917 & 0.919 & 0.929 & 0.898 & 0.919 & 0.858 & 0.936 & 0.952 & 0.917 & 0.928 & 0.813 & 0.924 & 0.876 \\ 
   \hline
\end{tabular}
\caption{Comparison of different methods for regional level \%ILI estimation in Region 7.  The RMSE, MAE, and correlation measures are reported. The method with the best performance is highlighted in boldface for each metric in each period. \label{tab:reg7}} 
\end{adjustwidth}\end{table*}
% latex table generated in R 4.0.1 by xtable 1.8-4 package
% Tue May  2 13:07:15 2023
\begin{table*}\begin{adjustwidth}{0cm}{0cm} \tiny
\centering
\begin{tabular}{c|llllllllllllllll}
  \hline
  & '09-'23 & '09-'15 & '09-'10 & '10-'11 & '11-'12 & '12-'13 & '13-'14 & '14-'15 & '15-'16 & '16-'17 & '17-'18 & '18-'19 & '19-'20 & '20-'21 & '21-'22 & '22-'23 \\ 
  \hline \hline \multicolumn{1}{l}{RMSE}\\ARGO-C & \textbf{0.307} & \textbf{0.336} & \textbf{0.812} & 0.237 & \textbf{0.152} & \textbf{0.213} & 0.283 & \textbf{0.294} & \textbf{0.132} & 0.351 & \textbf{0.169} & \textbf{0.470} & \textbf{0.361} & 0.134 & \textbf{0.244} & \textbf{0.710} \\ 
  ARGO2 & 0.319 & 0.347 & 0.831 & \textbf{0.219} & 0.169 & 0.252 & 0.300 & 0.323 & 0.151 & \textbf{0.337} & 0.172 & 0.476 & 0.415 & 0.139 & 0.259 & 0.758 \\ 
  VAR1 & 0.392 & 0.410 & 0.985 & 0.226 & 0.180 & 0.341 & 0.369 & 0.389 & 0.189 & 0.363 & 0.260 & 0.562 & 0.727 & \textbf{0.088} & 0.317 & 0.919 \\ 
  GFT & -- & 0.622 & 1.502 & 0.382 & 0.387 & 0.912 & \textbf{0.282} & 0.455 & -- & -- & -- & -- & -- & -- & -- & -- \\ 
  naive & 0.385 & 0.402 & 0.969 & 0.229 & 0.177 & 0.341 & 0.374 & 0.388 & 0.186 & 0.369 & 0.250 & 0.532 & 0.721 & 0.088 & 0.315 & 0.894 \\ 
   \hline \hline \multicolumn{1}{l}{MAE}\\ARGO-C & \textbf{0.177} & \textbf{0.172} & \textbf{0.403} & 0.189 & \textbf{0.105} & \textbf{0.161} & \textbf{0.169} & \textbf{0.199} & \textbf{0.109} & 0.262 & \textbf{0.130} & \textbf{0.372} & \textbf{0.262} & 0.105 & \textbf{0.187} & \textbf{0.554} \\ 
  ARGO2 & 0.182 & 0.177 & 0.411 & 0.181 & 0.117 & 0.170 & 0.177 & 0.225 & 0.121 & \textbf{0.250} & 0.132 & 0.376 & 0.290 & 0.114 & 0.195 & 0.595 \\ 
  VAR1 & 0.212 & 0.196 & 0.496 & \textbf{0.156} & 0.130 & 0.234 & 0.217 & 0.227 & 0.150 & 0.269 & 0.193 & 0.427 & 0.516 & \textbf{0.072} & 0.242 & 0.734 \\ 
  GFT & -- & 0.315 & 0.863 & 0.273 & 0.339 & 0.506 & 0.234 & 0.289 & -- & -- & -- & -- & -- & -- & -- & -- \\ 
  naive & 0.211 & 0.199 & 0.512 & 0.162 & 0.124 & 0.241 & 0.226 & 0.239 & 0.147 & 0.273 & 0.179 & 0.397 & 0.513 & 0.072 & 0.236 & 0.720 \\ 
   \hline \hline \multicolumn{1}{l}{Correlation}\\ARGO-C & \textbf{0.976} & \textbf{0.959} & 0.947 & 0.952 & \textbf{0.905} & \textbf{0.983} & 0.921 & \textbf{0.968} & \textbf{0.969} & 0.824 & 0.986 & \textbf{0.952} & \textbf{0.985} & 0.871 & \textbf{0.939} & \textbf{0.957} \\ 
  ARGO2 & 0.974 & 0.957 & 0.945 & \textbf{0.961} & 0.885 & 0.978 & 0.910 & 0.964 & 0.960 & \textbf{0.833} & \textbf{0.986} & 0.950 & 0.979 & 0.870 & 0.921 & 0.950 \\ 
  VAR1 & 0.960 & 0.938 & 0.923 & 0.941 & 0.874 & 0.955 & 0.866 & 0.930 & 0.931 & 0.797 & 0.963 & 0.924 & 0.933 & \textbf{0.891} & 0.848 & 0.917 \\ 
  GFT & -- & 0.859 & \textbf{0.988} & 0.929 & 0.872 & 0.926 & \textbf{0.955} & 0.930 & -- & -- & -- & -- & -- & -- & -- & -- \\ 
  naive & 0.961 & 0.941 & 0.927 & 0.941 & 0.877 & 0.955 & 0.867 & 0.931 & 0.935 & 0.803 & 0.963 & 0.930 & 0.935 & 0.889 & 0.848 & 0.915 \\ 
   \hline
\end{tabular}
\caption{Comparison of different methods for regional level \%ILI estimation in Region 8.  The RMSE, MAE, and correlation measures are reported. The method with the best performance is highlighted in boldface for each metric in each period. \label{tab:reg8}} 
\end{adjustwidth}\end{table*}
% latex table generated in R 4.0.1 by xtable 1.8-4 package
% Tue May  2 13:07:15 2023
\begin{table*}\begin{adjustwidth}{0cm}{0cm} \tiny
\centering
\begin{tabular}{c|llllllllllllllll}
  \hline
  & '09-'23 & '09-'15 & '09-'10 & '10-'11 & '11-'12 & '12-'13 & '13-'14 & '14-'15 & '15-'16 & '16-'17 & '17-'18 & '18-'19 & '19-'20 & '20-'21 & '21-'22 & '22-'23 \\ 
  \hline \hline \multicolumn{1}{l}{RMSE}\\ARGO-C & \textbf{0.347} & \textbf{0.437} & 0.665 & 0.358 & \textbf{0.382} & \textbf{0.474} & \textbf{0.297} & \textbf{0.284} & \textbf{0.224} & 0.199 & \textbf{0.404} & 0.181 & 0.306 & 0.135 & \textbf{0.229} & \textbf{0.639} \\ 
  ARGO2 & 0.359 & 0.453 & \textbf{0.654} & \textbf{0.353} & 0.394 & 0.525 & 0.319 & 0.330 & 0.244 & \textbf{0.186} & 0.413 & \textbf{0.178} & \textbf{0.288} & \textbf{0.134} & 0.250 & 0.700 \\ 
  VAR1 & 0.406 & 0.470 & 0.664 & 0.395 & 0.419 & 0.538 & 0.382 & 0.380 & 0.315 & 0.208 & 0.622 & 0.224 & 0.462 & 0.137 & 0.353 & 0.877 \\ 
  GFT & -- & 1.091 & 1.101 & 1.168 & 0.567 & 2.536 & 0.593 & 0.540 & -- & -- & -- & -- & -- & -- & -- & -- \\ 
  naive & 0.405 & 0.475 & 0.676 & 0.382 & 0.438 & 0.544 & 0.385 & 0.382 & 0.312 & 0.210 & 0.606 & 0.222 & 0.461 & 0.139 & 0.358 & 0.828 \\ 
   \hline \hline \multicolumn{1}{l}{MAE}\\ARGO-C & \textbf{0.213} & \textbf{0.275} & 0.502 & \textbf{0.261} & \textbf{0.308} & \textbf{0.325} & \textbf{0.204} & \textbf{0.201} & \textbf{0.172} & \textbf{0.142} & \textbf{0.265} & 0.132 & 0.230 & 0.109 & \textbf{0.183} & \textbf{0.453} \\ 
  ARGO2 & 0.217 & 0.282 & \textbf{0.488} & 0.270 & 0.321 & 0.339 & 0.214 & 0.219 & 0.186 & 0.149 & 0.266 & \textbf{0.127} & \textbf{0.209} & 0.109 & 0.184 & 0.480 \\ 
  VAR1 & 0.247 & 0.297 & 0.510 & 0.320 & 0.349 & 0.327 & 0.247 & 0.258 & 0.243 & 0.161 & 0.357 & 0.181 & 0.338 & \textbf{0.106} & 0.214 & 0.726 \\ 
  GFT & -- & 0.690 & 0.995 & 1.090 & 0.500 & 1.296 & 0.393 & 0.410 & -- & -- & -- & -- & -- & -- & -- & -- \\ 
  naive & 0.247 & 0.299 & 0.514 & 0.298 & 0.368 & 0.354 & 0.253 & 0.260 & 0.244 & 0.167 & 0.365 & 0.182 & 0.333 & 0.107 & 0.221 & 0.656 \\ 
   \hline \hline \multicolumn{1}{l}{Correlation}\\ARGO-C & \textbf{0.956} & \textbf{0.921} & 0.891 & \textbf{0.944} & 0.768 & \textbf{0.922} & \textbf{0.963} & \textbf{0.967} & \textbf{0.965} & 0.945 & \textbf{0.959} & 0.972 & 0.971 & 0.948 & \textbf{0.957} & \textbf{0.959} \\ 
  ARGO2 & 0.953 & 0.915 & 0.893 & 0.944 & 0.751 & 0.902 & 0.958 & 0.960 & 0.960 & \textbf{0.946} & 0.955 & \textbf{0.974} & \textbf{0.974} & \textbf{0.949} & 0.946 & 0.947 \\ 
  VAR1 & 0.940 & 0.909 & 0.887 & 0.922 & 0.728 & 0.894 & 0.925 & 0.930 & 0.930 & 0.933 & 0.897 & 0.957 & 0.929 & 0.943 & 0.887 & 0.895 \\ 
  GFT & -- & 0.806 & \textbf{0.945} & 0.905 & \textbf{0.844} & 0.900 & 0.937 & 0.917 & -- & -- & -- & -- & -- & -- & -- & -- \\ 
  naive & 0.941 & 0.910 & 0.890 & 0.924 & 0.728 & 0.894 & 0.926 & 0.931 & 0.933 & 0.933 & 0.901 & 0.958 & 0.930 & 0.942 & 0.886 & 0.896 \\ 
   \hline
\end{tabular}
\caption{Comparison of different methods for regional level \%ILI estimation in Region 9.  The RMSE, MAE, and correlation measures are reported.. The method with the best performance is highlighted in boldface for each metric in each period. \label{tab:reg9}} 
\end{adjustwidth}\end{table*}
% latex table generated in R 4.0.1 by xtable 1.8-4 package
% Tue May  2 13:07:15 2023
\begin{table*}\begin{adjustwidth}{0cm}{0cm} \tiny
\centering
\begin{tabular}{c|llllllllllllllll}
  \hline
  & '09-'23 & '09-'15 & '09-'10 & '10-'11 & '11-'12 & '12-'13 & '13-'14 & '14-'15 & '15-'16 & '16-'17 & '17-'18 & '18-'19 & '19-'20 & '20-'21 & '21-'22 & '22-'23 \\ 
  \hline \hline \multicolumn{1}{l}{RMSE}\\ARGO-C & \textbf{0.383} & \textbf{0.419} & 0.697 & 0.466 & 0.225 & \textbf{0.379} & \textbf{0.376} & \textbf{0.259} & \textbf{0.254} & \textbf{0.438} & \textbf{0.345} & \textbf{0.282} & \textbf{0.453} & 0.122 & 0.205 & \textbf{1.144} \\ 
  ARGO2 & 0.396 & 0.428 & \textbf{0.687} & 0.469 & \textbf{0.221} & 0.406 & 0.399 & 0.267 & 0.259 & 0.452 & 0.350 & 0.308 & 0.530 & 0.120 & \textbf{0.179} & 1.194 \\ 
  VAR1 & 0.471 & 0.469 & 0.733 & 0.477 & 0.235 & 0.438 & 0.463 & 0.330 & 0.277 & 0.493 & 0.504 & 0.410 & 0.774 & \textbf{0.085} & 0.267 & 1.526 \\ 
  GFT & -- & 1.083 & 0.800 & \textbf{0.423} & 0.629 & 2.880 & 0.869 & 0.339 & -- & -- & -- & -- & -- & -- & -- & -- \\ 
  naive & 0.457 & 0.457 & 0.705 & 0.493 & 0.237 & 0.451 & 0.467 & 0.325 & 0.271 & 0.506 & 0.505 & 0.400 & 0.783 & 0.085 & 0.259 & 1.393 \\ 
   \hline \hline \multicolumn{1}{l}{MAE}\\ARGO-C & \textbf{0.223} & \textbf{0.253} & 0.513 & 0.340 & \textbf{0.174} & \textbf{0.254} & \textbf{0.221} & \textbf{0.177} & \textbf{0.201} & \textbf{0.282} & 0.241 & \textbf{0.208} & \textbf{0.340} & 0.094 & 0.170 & \textbf{0.751} \\ 
  ARGO2 & 0.225 & 0.256 & 0.494 & 0.325 & 0.179 & 0.260 & 0.226 & 0.187 & 0.206 & 0.282 & \textbf{0.220} & 0.232 & 0.380 & 0.091 & \textbf{0.144} & 0.759 \\ 
  VAR1 & 0.253 & 0.260 & \textbf{0.454} & \textbf{0.306} & 0.202 & 0.263 & 0.270 & 0.245 & 0.213 & 0.282 & 0.292 & 0.282 & 0.569 & \textbf{0.063} & 0.185 & 1.184 \\ 
  GFT & -- & 0.644 & 0.610 & 0.355 & 0.597 & 2.175 & 0.764 & 0.254 & -- & -- & -- & -- & -- & -- & -- & -- \\ 
  naive & 0.255 & 0.270 & 0.474 & 0.335 & 0.208 & 0.286 & 0.280 & 0.248 & 0.208 & 0.330 & 0.321 & 0.277 & 0.564 & 0.064 & 0.176 & 0.997 \\ 
   \hline \hline \multicolumn{1}{l}{Correlation}\\ARGO-C & \textbf{0.958} & \textbf{0.944} & 0.964 & 0.869 & 0.852 & \textbf{0.920} & 0.926 & 0.959 & \textbf{0.903} & \textbf{0.880} & 0.962 & \textbf{0.968} & \textbf{0.969} & 0.900 & 0.932 & \textbf{0.937} \\ 
  ARGO2 & 0.956 & 0.942 & 0.964 & 0.866 & 0.860 & 0.905 & 0.916 & \textbf{0.960} & 0.899 & 0.872 & \textbf{0.962} & 0.962 & 0.958 & 0.906 & \textbf{0.946} & 0.930 \\ 
  VAR1 & 0.936 & 0.931 & 0.956 & 0.859 & 0.847 & 0.890 & 0.882 & 0.933 & 0.885 & 0.849 & 0.919 & 0.927 & 0.899 & \textbf{0.927} & 0.877 & 0.891 \\ 
  GFT & -- & 0.804 & \textbf{0.985} & \textbf{0.919} & \textbf{0.887} & 0.911 & \textbf{0.974} & 0.933 & -- & -- & -- & -- & -- & -- & -- & -- \\ 
  naive & 0.942 & 0.935 & 0.962 & 0.859 & 0.850 & 0.887 & 0.883 & 0.933 & 0.892 & 0.850 & 0.919 & 0.932 & 0.898 & 0.925 & 0.882 & 0.891 \\ 
   \hline
\end{tabular}
\caption{Comparison of different methods for regional level \%ILI estimation in Region 10.  The RMSE, MAE, and correlation measures are reported. The method with the best performance is highlighted in boldface for each metric in each period. \label{tab:reg10}} 
\end{adjustwidth}\end{table*}
